# Supplementary material for: Saddles, Twists, and Curls: Shape Transitions in Freestanding Nanoribbons
Source: arXiv:1107.3981 source file (2011-07-15)
Supplement: Supplementary file 1 [file SI.pdf]

# Supplementary Information for "Saddles, Twists, and Curls: Shape Transitions in Freestanding Nanoribbons"

Hailong Wang and Moneesh Upmanyu
*Group for Simulation and Theory of Atomic-Scale Material Phenomena (stAMP), Department of Mechanical and Industry Engineering, Northeastern University, Boston, Massachusetts 02115, USA.*

## I. ATOMISTIC SIMULATIONS

To facilitate direct comparison with past computational studies, we have performed these computations using a reactive bond order (AIREBO) potential as implemented in the software package LAMMPS [8]. The nanoribbons were perturbed by small curvature or twist and then relaxed to their equilibrium shape using a conjugate gradient algorithm with an energy tolerance of $10^{-10}$ eV. Figure S1 shows some equilibrium shapes of AGNRs as a function of their width, in addition to the shapes shown in Fig. 1 in the text. Note the combined saddle-like and edge rippled morphology for the $w = 19.97$ nm ribbon. The edge ripples are also observed at the ends of the ribbon with width $w = 9.91$ nm.

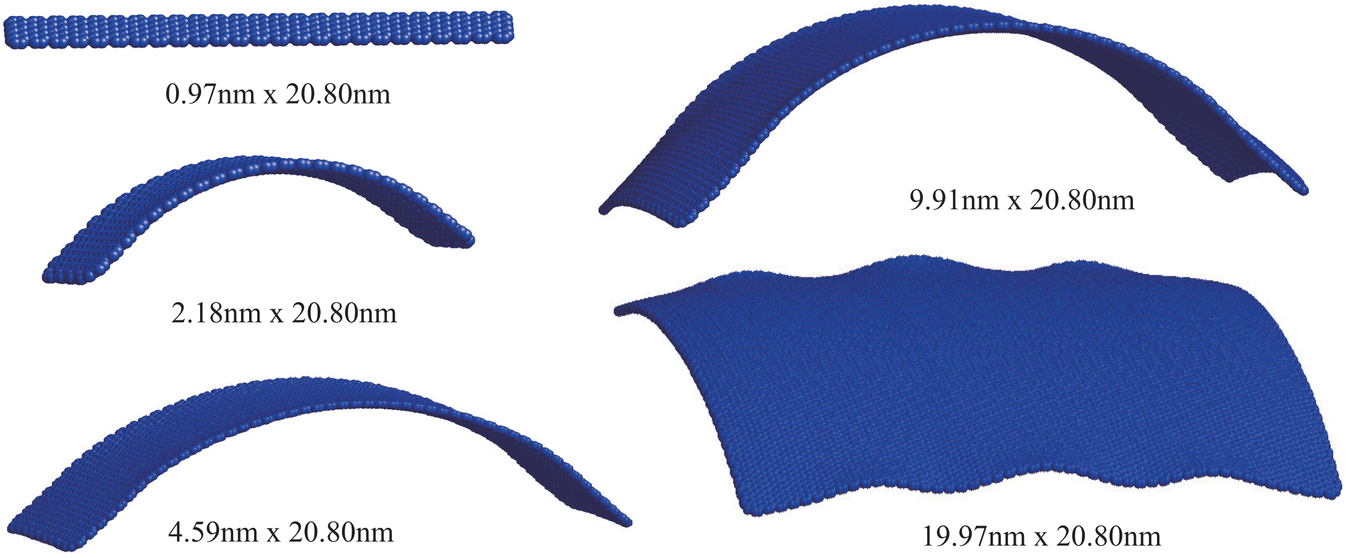


Figure S1: Saddle-like shapes of armchair graphene nanoribbons with different width obtained by relaxing graphene with curvature using the AIREBO potential.

The simulations for the tapered nanoribbon shown in Fig. 3c in the text are also performed similarly. The equilibrium longitudinal curvature $\kappa(s)$ that is used to color-code the equilibrated shape is based on the shape of the ribbon midline which is readily available from the computations.

## II. COMPOSITE CORE-EDGE FRAMEWORK

The nanoribbon core is modeled as an infinite linear isotropic elastic thin plate with thickness $h$, width $w$, and length $l$ ($h \ll w \ll l$). In the limit of small strains, the out-of-plane deflections are governed by the classical Föppl-von-Kármán equations [6],

$$D\nabla^4\zeta = \Phi_{,yy}\zeta_{,xx}$$
$$\nabla^4\Phi = -S(\zeta_{,xx}\zeta_{,yy} - \zeta_{,xy}^2) \tag{S1}$$

where $\Phi$ is the Airy function associated with the in-plane stresses and the operator $\nabla^4 A = A_{,xxxx} + 2A_{,xxyy} + A_{,yyyy}$. For long lengths, the mid-surface forces per unit length $N_y$ and $N_{xy}$ are negligible and can be safely ignored. Then,

the out-of-plane deflections $\zeta$ are due to the longitudinal force, or ribbon tension, $T = N_x$, and the F-vK equations reduce to Eqs. 1-2 in the main text.

The highly localized edge is assumed to be elastic string glued to the ribbon core and stretched or compressed in accordance with the sign of the edge stress. For a ribbon so structured, we must account for the longitude strain compatibility between the plate boundary and edge string (Eq. 3 in text),

$$\epsilon_{xx}(\pm\frac{w}{2}) = T(\pm\frac{w}{2})/S = (\tau_e^{\pm} - \tau_e)/S_e, \tag{S2}$$

where $\tau_e^{\pm}$ is residual edge stress as defined in the text. Free torques and zero shear force balance serve as boundary conditions that complete the formulation. Setting our origin on the ribbon centerline, we get

$$\begin{aligned} \{\zeta_{,yy} + \nu\zeta_{,xx}\}|_{\pm\frac{w}{2}} &= 0, \\ \{\zeta_{,yyy} + (2-\nu)\zeta_{,yxx}] \pm \frac{\tau_e}{D}\zeta_{,xx}\}|_{\pm\frac{w}{2}} &= 0. \end{aligned} \tag{S3}$$

Note that Eq. 1 and Eq. S3 satisfy the global in-plane force equilibrium along the longitudinal direction $\int_{-w/2}^{w/2} T\,dy + (\tau_e^- + \tau_e^+) = 0$ and the global torque equilibrium in the transverse direction $\int_{-w/2}^{w/2} T\,ydy + (\tau_e^+ - \tau_e^-)w/2 = 0$.

## III. GENERAL SOLUTION: RIBBON SHAPE AND ENERGETICS

The shallow-shell ansatz (Eq. 3 in the main text) is motivated by the saddle-like/curled and twisted shapes observed in the computations. Substituting in Eq. 1 and Eq. S3 yields the boundary value problem for the shape function, $f$ (Eq. 5 in the text). The constants associated with the solution (Eq. 6 in the text) are

$$\begin{aligned} C_1 &= \sqrt{\frac{D}{S}}\frac{2\phi(\nu+\theta^2/\kappa^2)(\sinh\phi\cos\phi - \cosh\phi\sin\phi) - \bar{\tau}_e\cosh\phi\cos\phi - 8\phi^2\bar{S}_e(\nu+\theta^2/\kappa^2)\sinh\phi\sin\phi}{4\phi^2\bar{S}_e(\cosh 2\phi + \cos 2\phi) + \phi(\sinh 2\phi + \sin 2\phi)} \\ C_2 &= \sqrt{\frac{D}{S}}\frac{2\phi(\nu+\theta^2/\kappa^2)(\sinh\phi\cos\phi + \cosh\phi\sin\phi) - \bar{\tau}_e\sinh\phi\sin\phi + 8\phi^2\bar{S}_e(\nu+\theta^2/\kappa^2)\cosh\phi\cos\phi}{4\phi^2\bar{S}_e(\cosh 2\phi + \cos 2\phi) + \phi(\sinh 2\phi + \sin 2\phi)} \\ C_3 &= \sqrt{\frac{D}{S}}\left[\frac{1}{48}\frac{\bar{\theta}^2}{k^2w^2} + \frac{\bar{\tau}_e/(4\phi)(\sinh 2\phi + \sin 2\phi) + 2\phi\bar{S}_e(\nu+\theta^2/\kappa^2)(\sinh 2\phi - \sin 2\phi)}{4\phi^2\bar{S}_e(\cosh 2\phi + \cos 2\phi) + \phi(\sinh 2\phi + \sin 2\phi)}\right] \end{aligned} \tag{S4}$$

where $\phi$ and $k$ are related to the longitudinal curvature as $4\phi^2 = (kw)^2 = \bar{\kappa}/2$. The constant $C_3$ is selected so as to remove the translational and rotational freedom, i.e. $\int_{-\frac{w}{2}}^{\frac{w}{2}} f(y)dy = 0$. The scaled variables that appear in these and following expressions are as defined in the main text.

The equilibrium ribbon shape also yields the excess elastic energy $\delta\mathcal{E}(\theta,\phi)$, defined with respect to an initially flat ribbon ($\mathcal{E}(0,0) = 0$), with contributions from bending and stretching of the core ($\mathcal{E}_b$ and $\mathcal{E}_s$, respectively), and stretching at the edges ($\mathcal{E}_s^e$), where

$$\begin{aligned} \mathcal{E}_b &= \frac{D}{2}\int(\frac{\partial^2\zeta}{\partial x^2} + \frac{\partial^2\zeta}{\partial y^2})^2 + 2(1-\nu)[(\frac{\partial^2\zeta}{\partial x\partial y})^2 - \frac{\partial^2\zeta}{\partial x^2}\frac{\partial^2\zeta}{\partial y^2}]dy \\ \mathcal{E}_s &= \frac{1}{2S}\int {N_x}^2 dy \\ \mathcal{E}_s^e &= {\tau_e}^-\epsilon_e^- + \frac{1}{2}S_e{\epsilon_e^-}^2 + {\tau_e}^+\epsilon_e^+ + \frac{1}{2}S_e{\epsilon_e^+}^2 \end{aligned} \tag{S5}$$

## IV. PURE TWIST ($\tau_e < 0$)

The solution for the equilibrium ribbon twist (Eq. 7 in the text) follows from the general solution, in the limit $\kappa \to 0$. In terms of unscaled variables, the solution for the ribbon tension and the the post-buckled edge stress are,

$$\begin{aligned} f &= 0 \\ T &= S[\frac{1}{2}\theta^2y^2 - \frac{48\tau_e + (Sw + 6S_e)\theta^2w^2}{24(Sw + 2S_e)}] \\ \tau_e^{\pm} &= \tau_e + S_e(\frac{1}{8}\theta^2w^2 - \frac{2\tau + \theta^2w^2(S_e/4 + Sw/24)}{Sw + 2S_e}) \end{aligned} \tag{S6}$$

The equilibrium twist $\theta_{eq}$ (Eq. 7 in the text) and the related critical edge stress ($\bar{\tau}_e^* = -6(1-\nu)(1+\bar{S}_e)$) are determined by enforcing zero net torque along the longitudinal direction, $T = \partial\mathcal{E}/\partial\theta = 0$. The excess energy associated with the twisted ribbon is

$$\delta\mathcal{E} = -\frac{10[S\tau_e w^2 + 6D(1-\nu)(2S_e + Sw)]^2}{Sw^3(2S_e + Sw)(12Se + Sw)} \tag{S7}$$

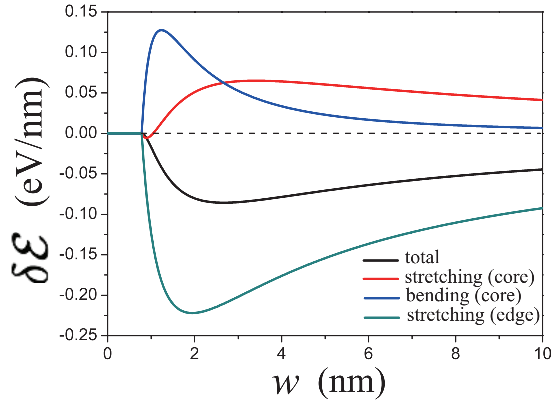


Figure S2: Width variation of the excess energy for equilibrium twisted AGNRs ($\tau_e = -10.5\,\mathrm{eV/nm}$) corresponding to Fig. 2a in the main text. The variation in the energies stored in stretching (core and edge) and bending (core) are also shown.

Figure S1 shows the variation in the energy for pristine AGNRs with edge stress $\tau_e = -10.5\,\mathrm{eV/nm}$. At the onset of buckling, the equilibrium shape is mainly due to a competition between bending of the core and stretching of the edge. However, at large widths, the stretching of the core and edge dominate the energetics. This is also evident from the analytical solution for the excess energy, in the limit of large width and/or large in-plane stiffness, as for example in the case of GNRs ($w \gg S_e/S$ and $w \gg -D/\tau_e$). Then, we arrive at the following scaling for the twist (Eq. S7) and the energy,

$$\theta = 2\sqrt{30}(-\tau_e)^{\frac{1}{2}} S^{-\frac{1}{2}} w^{-\frac{3}{2}} \tag{S8}$$

$$\begin{aligned}
\delta\mathcal{E} &= -10\tau_e^2 S^{-1} w^{-1} \\
\mathcal{E}_s &= 10\tau_e^2 S^{-1} w^{-1} \\
\mathcal{E}_b &= 120(1-\nu)\tau_e D S^{-1} w^{-2} \\
\mathcal{E}_e &= -20\tau_e^2 S^{-1} w^{-1}.
\end{aligned} \tag{S9}$$

## V. BENDING: SADDLE-LIKE ($\tau_e < 0$) AND CURLED ($\tau_e > 0$) SHAPES

The equilibrium longitudinal curvatures $\kappa_{eq}$ for bent ribbons and can be obtained by setting $\theta \to 0$ in Eq. 5 in the text. The full solution (plotted in Fig. 2b of the text for AGNRs with pristine and reconstructed edges) is lengthy, and for compactness, we report the results in the limit $w \gg S_e/S$ ($\bar{S}_e \to 0$). The constants C1-C3 are available from Eq. S4 by setting $\theta = 0$ which in turn yield the excess energy associated with a bent ribbon (Eq. S5),

$$\delta\mathcal{E} = \frac{D^2 kw}{Sw^3} \frac{k^3w^3(\sin kw + \sinh kw) - \bar{\tau}_e^2(\cos kw + \cosh kw) + 2\nu^2 kw[kw(\cos kw - \cosh kw) + \nu\bar{\tau}_e(\sinh kw - \sin kw)]}{(\sin kw + \sinh kw)},$$

where the $kw$ is related to the (scaled) curvature as before, $(kw)^2 = \bar{\kappa}/2$. The bending moment along the longitudinal direction must vanish at equilibrium, $\partial\mathcal{E}/\partial\kappa = 0$, and yields the equilibrium curvature $\kappa_{eq}$. The resultant equation is

$$\bar{\tau}_e = \frac{-b \pm \sqrt{b^2 - 4ac}}{2a}, \quad \text{where} \tag{S10}$$

$$\begin{aligned}
a &= 4kw + \cos kw(4kw\cos kw - 2\sin kw) - \sin 2kw - 2\cos kw \sinh kw - \sinh 2kw \\
b &= 4\nu kw(-2 + \cos 2kw + \cosh 2kw + 2kw\cosh kw \sin kw - 2kw\cos kw \sinh kw) \\
c &= 2k^2w^2\{-2kw\cos 2kw + 6\nu^2(\cos kw - \cosh kw)(\sin kw + \sinh kw) + 2kw[\cosh 2kw + 2(2-\nu^2)\sin kw \sinh kw]\}
\end{aligned}$$

For small curvature such that $kw \to 0$, the scaled critical edge stress associated with the bent ribbon simplifies to

$$\bar{\tau}_e^* = \sqrt{5}(\sqrt{5}\nu \pm \sqrt{6-\nu^2}), \tag{S11}$$

as reported in the text. Note that for non-zero $\bar{S}_e$, the critical stress is amplified by the factor $1 + 2\bar{S}_e$. At large curvatures such that $kw \gg 1$, we get $\bar{\tau}_e^* = \pm 2\sqrt{k^3 w^3}$, which leads to the following scalings for the longitudinal curvature and the energies,

$$\kappa = \frac{1}{2^{1/3}} \frac{|\tau_e|^{4/3}}{S^{1/2} D^{5/6} w^{2/3}} \tag{S12}$$

$$\begin{aligned}
\delta\mathcal{E} &= -\frac{3}{2^{5/3}} |\tau_e|^{8/3} S^{-1} D^{-2/3} w^{-1/3} \\
\mathcal{E}_s &= \frac{3}{2^{5/3}} |\tau_e|^{8/3} S^{-1} D^{-2/3} w^{-1/3} \\
\mathcal{E}_b &= \frac{1}{2^{3/2}} |\tau_e|^{8/3} S^{-1} D^{-2/3} w^{-1/3} \\
\mathcal{E}_e &= -2^{4/3} |\tau_e|^{8/3} S^{-1} D^{-2/3} w^{-1/3}
\end{aligned} \tag{S13}$$

The prefactors in the energy scalings are $-0.945$, $0.945$, $0.630$ and $-2.520$. Similar scaling laws have also been reported in recent work on spontaneous curling of reconstructed AGNR [7]. However, it ignores the interplay between the boundary conditions and force balance along the longitudinal and transverse directions. Furthermore, the initial bifurcation in $\kappa_{eq}$ versus $w$ is ignored because the critical width for the reconstructed AGNRs $w^* < 0.5$ nm, based on our predictions.

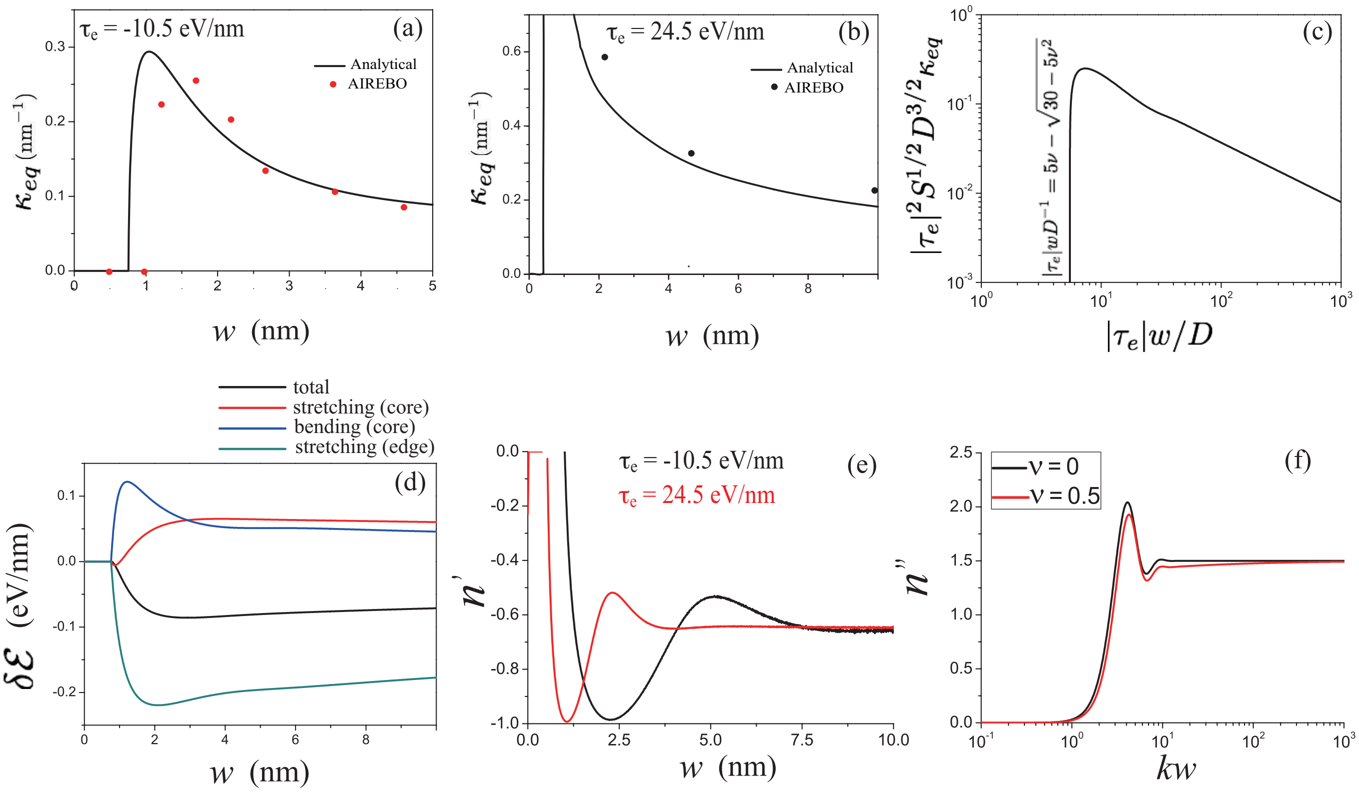


Figure S3: (a-b) The width dependence of the equilibrium curvatures observed in all atom simulations and those predicted by our composite framework, for pristine and reconstructed AGNRs ($\tau_e = -10.4$ eV/nm and $\tau_e = 24.5$ eV/nm). (c) Scaled plot, similar to the that shown in the inset in Fig. 2b, plotted in the limit $S_e = 0$. (d) Width dependence of the energetics associated with equilibrium saddle-like shapes predicted by the composite framework. (e-f) The variation in the two exponents, $n'$ and $n''$, with width. (e) $n'$ is the width exponent, $\kappa_{eq} = w^{n'}$ and it variation is plotted for pristine and reconstructed AGNRs, (f) and $n''$ relates the equilibrium curvature to the wavenumber, $\kappa_{eq} = (kw)^{n''}$. The two curves illustrate negligible effect of the Poisson's ratio $\nu$.

Figures S3a and S3b shows the comparison between the atomic-scale simulations and the predictions of our composite framework for the width dependence equilibrium curvatures for pristine and reconstructed AGNRs. The agreement between the two extends to near the bifurcation point (Fig. S3a) and large widths. Figure S3c shows a representative scaled plot in the limit $S_e = 0$ for tensile and compressive edge stress. The critical edge stress is now dependent on the Poisson's ratio, as indicated, and the large width behavior is as reported in the main text. The deviations in the scalings at intermediate values of the (scaled) edge stress (near the peak) indicate a departure from the scaling for the equilibrium curvature (Eq. S12) and also in the underlying energetics; this latter is evident from the variation in the energy (total as well as those stored in the core and edge) plotted in Fig. S3d. As in the case of twist, the stretching has a minor role to play at the onset of bucking, but becomes increasingly important at larger widths. To quantify this departure, Fig S3e and S3f show the width dependence of two exponents related to $n$ in the main text - $n'$ associated with $\kappa_{eq}$ vs. $w$, and $n''$ associated with $\bar{\tau}_e$ vs. $kw$. The oscillations observed in the exponent have little to do with the finite edge modulus $S_e$ (the scaled plot is for $S_e = 0$) or the Poisson's ratio (Fig. S3f) and indicate a non-trivial effect associated with changes in the ribbon profile (Fig. 2c and 2d in the text), i.e the edge-edge interactions at intermediate widths give way to ribbon shapes with well defined and stretched boundary layers separated by an almost flat midsection.

## VI. COMBINED BENDING AND TWIST

Figure S4a shows the contour plot of the excess elastic energy per unit length $\delta\mathcal{E}$ for a hypothetical GNR with tensile edge stress $\tau_e = 10.5eV$ and width $w = 3\,\mathrm{nm}$, similar to the plot showed in Fig. 3a in the main text. As expected, the twist becomes untenable for ribbons with tensile edge stress. However, the energy difference between pure bending and a combined shape with a small twist is not significant and can be easily overcome at room temperature. Figure S4b shows a similar contour plot, but for a pristine AGNR with width $w = 10\,\mathrm{nm}$. Comparison with the plot shown in Fig. 3a in the main text allows us to quantify the effect of width on such combined shapes. The excess energy decreases in its absolute value as the width increase and pure bending becomes more favorable.

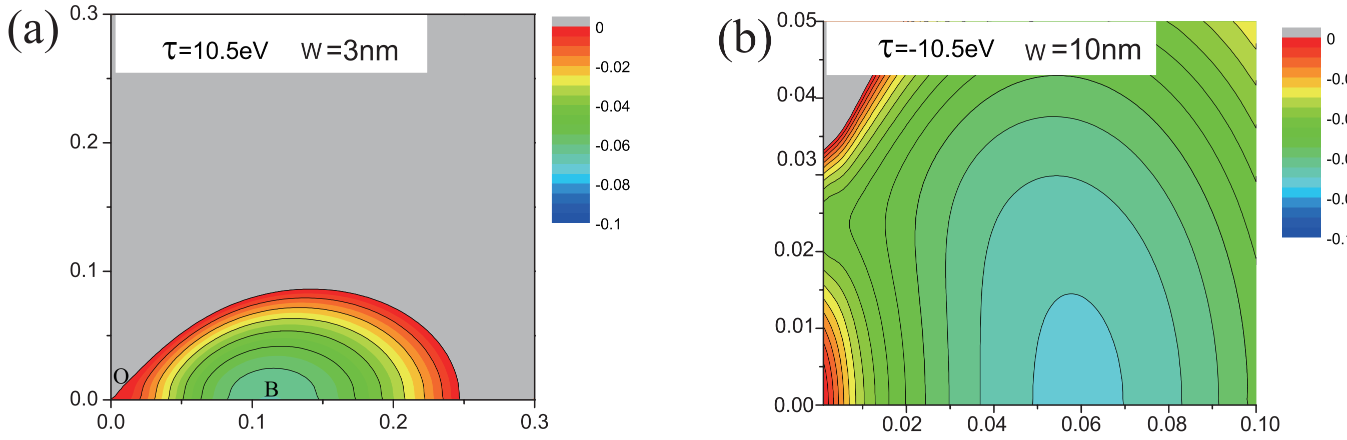


Figure S4: (a) Contour plot of the the excess elastic energy per unit length associated with combined bending and twist of (a) a hypothetical GNR with tensile edge stress $\tau_e = 10.5eV$ and width $w = 3\,\mathrm{nm}$, and (b) pristine AGNRs with compressive edge stress $\tau_e = -10.5eV$ and $w = 10nm$. The plots are similar to the contour plot shown in Fig. 3; the energy unit is eV/nm and the gray regions indicate flat ribbon profiles due to positive excess energy.

## VII. TRANSITION TO EDGE RIPPLING

At much larger widths, the bent shapes transition to rippled shapes - edge rippling for compressive edge stresses and midline dimpling in the case of tensile edge stresses. Our simulations indicate that the transition is likely gradual involving intermediate coexisting shapes that are rippled and bent, as seen in Fig. S1. A general treatment of the post-buckled shapes is beyond the scope of the present study, but past theoretical and computational studies offer some insight into the widths into the transition widths for GNRs. Following Ref. [1], we assume a sinusoidal edge warping with displacement $\zeta(x, y) = A\sin(kx)e^{-y/l}$ of amplitude $A$ and wavelength $\lambda = 2\pi/k$, where $l$ denotes the

length-scale over which the ripples penetrate into the sheet. Minimization of strain energy, assumed to be mainly due to stretching, yields $l \approx 0.23\lambda$ and $A \approx \sqrt{(-\lambda\tau_e)/(1.37S + 14.8S_e/\lambda)}$. The total strain energy per period $2\pi/k$ is only dependent on the wave length $\lambda$ and was reported in Ref. [1] for semi-infinite graphene sheets, which we reproduce here for the sake of completeness,

$$\delta\mathcal{E} = \mathcal{E}_s = \frac{\pi\tau_e A^2 k}{2} + \frac{3\pi S_e A^4 k^3}{32} + \frac{S}{1-\nu^2}\frac{\pi A^4}{8}\frac{3k^4l^4 + 2k^2l^2 + 3}{16kl^3}. \tag{S14}$$

The wavelength dependence of the excess strain energy per unit length $\delta\mathcal{E}/\lambda$ as well as the related amplitude $A$ armchair and zigzag GNRs are shown in Fig. S5a. Note that the result is valid only for large amplitudes in the limit that the bending energy can be neglected compared to stretching energy. At small wavelengths (and therefore amplitudes), the energy minimum occurs at zero wave length and it is clear that one cannot obtain the most stable wave length based on minimization of the stretching energy, $d(\mathcal{E}_s)/d\lambda = 0$; this bending energy must be factored in into the energetics.

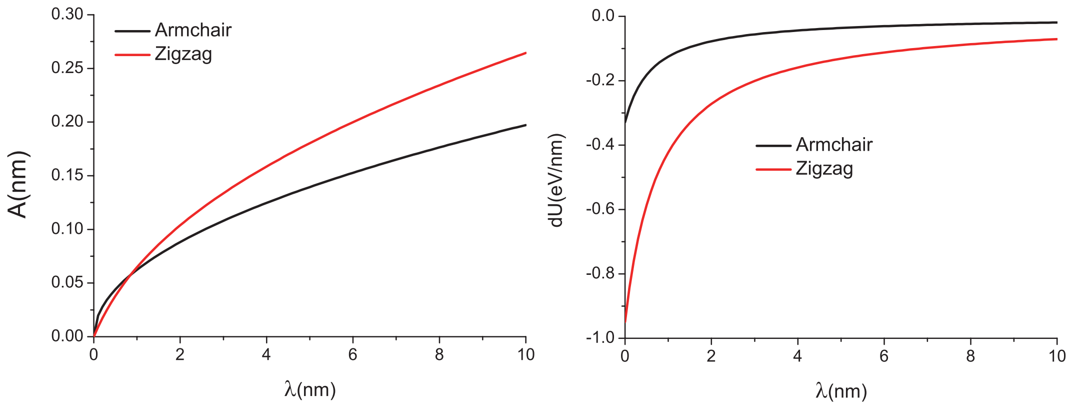


Figure S5: (a) The amplitude $A$ as a function of wave length $\lambda$ for edge rippling in armchair and zigzag GNRs. (b) The strain energy stored in stretching $\mathcal{E}_s$ as a function of wave length $\lambda$. All the plots are calculated from Eq. S14. See text for details.

In order to estimate the transition width associate with rippling, we use results from atomic-scale simulations performed by Bets and Yakobson, wherein the transition from twist to edge rippled shapes was found to obey the relation,

$$\lambda^* \approx -4\pi^2 D/\tau_e \tag{S15}$$

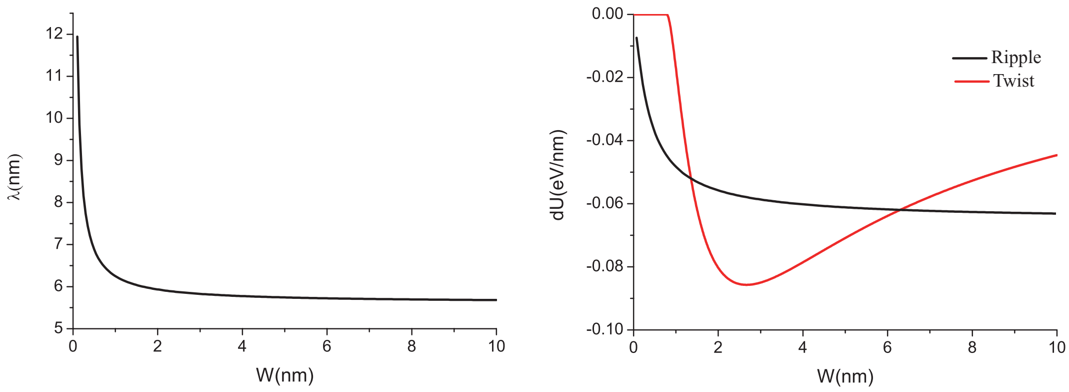


Figure S6: (a) Edge ripple amplitude of pristine AGNRs based on Eq. S14. (b) The excess energy for pure twist and edge ripples. The energy for edge rippling is again from Eq. S14 and that for pure twist is from the main text.

In the case of pristine AGNRs ($\tau_e = 10.5\,\mathrm{eV/nm}$ and $D = 1.5\,\mathrm{eV}$), we get $\lambda^* = 5.64\,\mathrm{nm}$. The amplitude is still large enough such that the bending energy can be ignored. In that limit, the energy released per unit length of two armchair edges follows from Eq. S14, $2\delta\mathcal{E}_s/\lambda = -6.66 \times 10^{-2}\,\mathrm{eV/nm}$. This energy estimate for the edge-rippling is plotted in Fig. 3b and yields the widths associated with the transition from saddle-like shapes to edge ripples shapes in pristine AGNRs. A similar analysis can be be used to predict the transition from curled shapes to dimpled shapes in systems with tensile edge stresses. As an example, the wave length and energy release is shown Fig. S6 for the transition of from global twist to edge rippling; the transition width is around 6 nm, also evident from the Fig. 3b.
